# Supplementary material for: Bifractality in one-dimensional Wolf-Villain model
Source: arXiv:2405.07133 source file (2024-05-12)
Supplement: Supplementary file 1 [file SM.pdf]

Supplementary Materials for

# Bifractality in one-dimensional Wolf-Villain model


Edwin E. Mozo Luis[1,⋆], Silvio C. Ferreira[2,3,†], and Thiago A. de Assis[4,1,‡]

[1]*Instituto de Física, Universidade Federal Fluminense,*

*Avenida Litorânea s/n, 24210-340, Niterói, RJ, Brazil*

[2]*Departamento de Física, Universidade Federal de Viçosa, Minas Gerais, 36570-900, Viçosa, Brazil*

[3]*National Institute of Science and Technology for Complex Systems, 22290-180, Rio de Janeiro, Brazil*

[4]*Instituto de Física, Universidade Federal da Bahia, Campus Universitário da Federação,*

*Rua Barão de Jeremoabo s/n, 40170-115, Salvador, BA, Brazil*

⋆emozo@id.uff.br

†silviojr@ufv.br

‡thiagoaa@ufba.br


## 1 Height difference correlation function

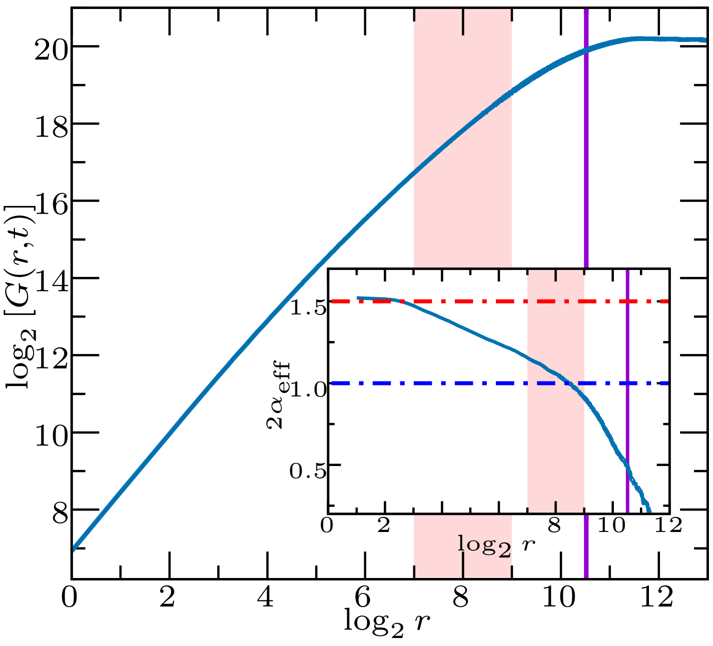


**Figure S1:** $\log_2[G(r,t)]$ vs. $\log_2 r$ at $t = 10^9$, considering the WV model in $d = 1$. Simulations were performed for $L = 2^{14}$ and data averaged over 400 independent realizations. The (red) highlighted region indicates a limit where the local roughness was extracted in Ref. [18] of the main text. Vertical (violet) filled line indicates the value of the correlation length $\xi_0 = 1462$ at $t = 10^9$. The inset shows $2\alpha_{\text{eff}} \equiv \frac{d \log_2[G(r,t)]}{d \log_2 r}$ vs. $\log_2 r$. The dash-dotted horizontal bottom (top) lines represents the values of 1 and $3/2$, respectively.

## 2 Autocorrelation function

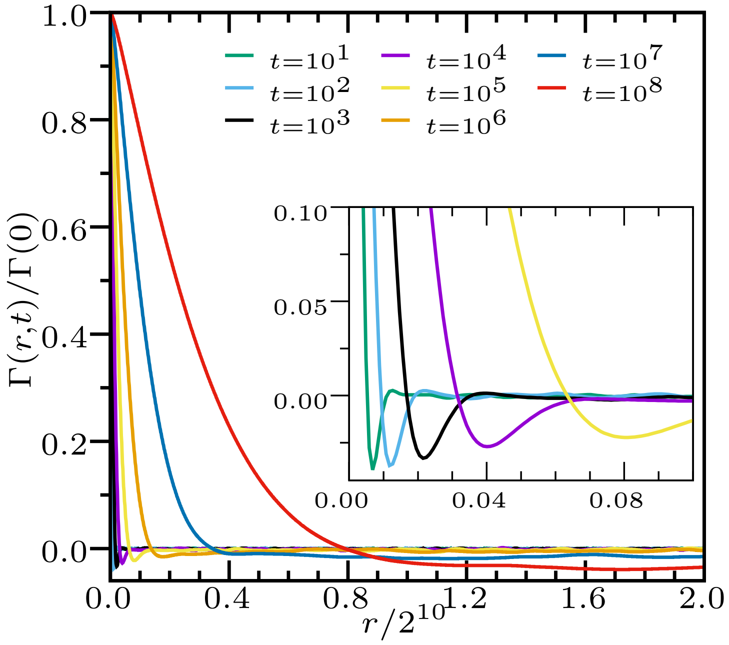


**Figure S2:** $\Gamma(r,t)/\Gamma(0)$ vs. r for different times, considering the WV model in $d = 1$. The inset shows the zoom for $\Gamma(r,t)/\Gamma(0) \leq 0.1$ and $10 \leq t \leq 10^5$.

## 3 MF-ODFA applied to the Restricted Solid on Solid (RSOS) model

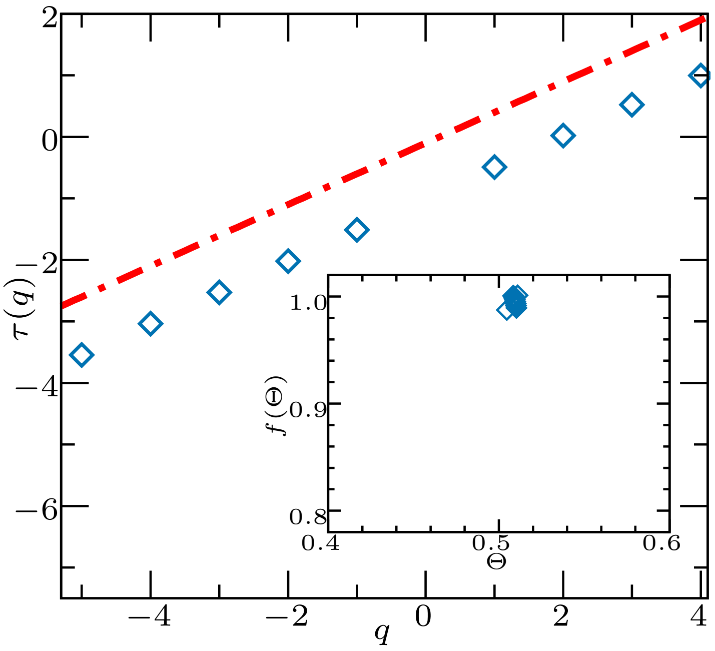


**Figure S3:** $\tau(q)$ vs. $q$ at $t = 5 \times 10^6$ for MF-ODFA analysis of the RSOS model in $d = 1$, with $n = 2$ and lateral size $L = 2^{15}$. Each point in the main panel represents the result of an average over 1000 independent realizations. The dashed line indicates the slope corresponding to the value of $\alpha$ for the Kardar-Parisi-Zhang class in $d = 1$. The inset shows $f(\Theta)$ vs. $\Theta$ for the case of the main panel.
